# Supplementary material for: Networks and Hierarchies: How Amorphous Materials Learn to Remember
Source: arXiv:1905.09259 ancillary file (2019-11-05)
Supplement: Supplementary file 1 [file Supplementary.pdf]

# Supplemental Material to "Networks and Hierarchies: How Amorphous Materials Learn to Remember"

Muhittin Mungan,[1,*] Srikanth Sastry,[2] Karin Dahmen,[3] and Ido Regev[4,†]

[1] *Institut für angewandte Mathematik, Universität Bonn, Endenicher Allee 60, 53115 Bonn, Germany*
[2] *Jawaharlal Nehru Centre for Advanced Scientific Research, Jakkar Campus, 560064 Bengaluru, India*
[3] *Department of Physics, University of Illinois at Urbana-Champaign, 1110 West Green Street, Urbana, IL 61801, USA*
[4] *Jacob Blaustein Institutes for Desert Research, Ben-Gurion University of the Negev, Sede Boqer Campus 84990, Israel*

(Dated: November 5, 2019)

## S1 NUMERICAL IMPLEMENTATION DETAILS OF MESOSTATE EXTRACTION, IDENTIFICATION AND CONSTRUCTION OF THE TRANSITION GRAPH

In this section we give further details about how we numerically identify mesostates and how these are used to construct their transition graph. This section is organized as follows. In S1.1 we show how we extract mesostates from the numerical simulation of the sheared amorphous solid. In S1.2 we describe how, given two mesostates, we determine whether they are identical or not. S1.3 presents the algorithm in pseudo code that we have used to gather a catalog of mesostates, using the numerical simulations to determine mesostate transitions. Finally, in S1.4 we provide a step-by-step example that illustrate this numerical procedure for a small catalog of mesostates. This example also shows how the mesostate transition graph is obtained from the catalog.

### S1.1 Mesostate extraction

Our approach is based on the concept of a "mesostate", which is applicable in the AQS regime of very slow driving and negligible thermal effects so that the system is always in a mechanically stable configuration. Consider a particle configuration $a_0$ (i.e. a vector of particle positions $\mathbf{r}$) that is stable at a strain $\gamma_0$. Increasing the strain by a small amount $\Delta\gamma$ while maintaining AQS conditions (i.e. keeping the potential energy at a local minimum) the system will undergo a small elastic deformation, reaching a new configuration stable at $\gamma_0 + \Delta\gamma$. We can keep increasing the strain in this way, allowing the configuration to adapt by small elastic deformations, until we reach a strain $\gamma^+$ where the local configuration is not locally stable anymore. This instability is manifested in a discontinuous drop in the potential energy and in the *i.e.* which is a result of a saddle node bifurcation which leads the system from one stable configuration to another. In terms of the displacement field, this instability causes a plastic rearrangement of particles changing their equilibrium positions. Similarly, starting at $a_0$ and decreasing the strain by small amounts $-\Delta\gamma$, we reach a strain value $\gamma^-$ where another plastic event occurs. Starting in $a_0$ at strain $\gamma_0$ and varying $\gamma$ between these values so that $\gamma^- < \gamma < \gamma^+$ for all times, the configuration undergoes purely elastic deformations that are reversible. For example, if we deform the material such that $\gamma$ returns to $\gamma_0$, the particle configuration also returns to $a_0$. Irreversible transitions can occur only when $\gamma > \gamma^+$ or $\gamma < \gamma^-$. We call the set of particle configurations containing $a_0$ at $\gamma_0$ and that can be transformed into each other purely elastically by varying the strain between $\gamma^-$ and $\gamma^+$ a *mesostate*. It is a set of particle configurations that transform reversibly into each other when varying the strain. We label the mesostate containing the configuration $a_0$ as $A$. The stability interval of $A$ is given by the two strains $\gamma^\pm$ and we write this as $(\gamma^-(A), \gamma^+(A))$.

In our numerical implementation we start with a stable configuration $a$ at strain $\gamma$. We then keep increasing the strain by an amount $\Delta\gamma$. After each strain increase, we recalculate the new stable configuration by minimizing the potential energy. We monitor the difference in energy $\Delta\mathcal{U}$ between the equilibrium locations at $\gamma$ and $\gamma + \Delta\gamma$. If $\Delta\mathcal{U} < 0$ decreases in a discontinuous manner (we check this by calculating the numerical derivative of $\mathcal{U}$) we conclude that a plastic event has occurred. We thereby obtain the value $\gamma^+(A)$. We determine $\gamma^-(A)$ in a similar manner, starting from $a$ at $\gamma$ and decreasing the strain by amounts of $-\Delta\gamma$ until a plastic event occurs. For the results reported in the paper, we used $\Delta\gamma = 10^{-4}$. Potential energy minimizations were performed using the FIRE algorithm. We have also repeated some of the simulations using the conjugate gradient method and found that the set of mesostates

* Corresponding author: mungan@iam.uni-bonn.de
† Corresponding author: regevid@bgu.ac.il

identified this way are nearly identical. Similarly, we also performed the same simulations using a smaller increment of $\Delta\gamma = 10^{-5}$, finding again that with a few and insignificant exceptions the same set of mesostates was extracted.

### S1.2 Mesostate identification

Starting at a particle configuration $a$ stable at strain $\gamma$, this configuration is part of some mesostate $A$, with stability interval $\gamma^-(A) < \gamma < \gamma^+(A)$. Increasing the strain to $\gamma^+(A)$ a plastic deformation occurs as a result of which we obtain a new particle configuration $b$ stable at $\gamma = \gamma^+(A)$. By our definition of mesostates, $b$ must belong to another mesostate, which we shall call $B$ with its stability interval $\gamma^\pm(B)$. Staring in $a$ at $\gamma$ and raising the strain to $\gamma^+(A)$, we have in effect triggered a mesostate transition $A \to B$. Similarly, starting again in $a$ at $\gamma$ and lowering the strain to $\gamma^-(A)$, a new configuration $c$ stable at $\gamma^-(A)$ is reached that belongs to some mesostate $C$. Mesostate transitions capture therefore plastic events. Moreover, from every mesostate $A$ there are two mesostate transitions, which we shall label $U$ and $D$, which occur when $\gamma$ is raised to $\gamma^+(A)$ or lowered to $\gamma^-(A)$, respectively.

By applying positive and negative strain to $B$ and $C$, we reach four more mesostates. These are the mesostates associated with the plastic events occurring at $\gamma^\pm(B)$ and $\gamma^\pm(C)$. Some of these resulting mesostates may or may not be equal to each other or they may be equal to some other mesostate obtained before. We thus need to be able to tell whether two given mesostates $X$ and $Y$ are identical or not. We make the following definition: two mesostates $X$ and $Y$ are equal if $\gamma^\pm(X) = \gamma^\pm(Y)$ and the microscopic configurations $x$ and $y$ at some common strain $\gamma$ with $\gamma^-(X) < \gamma < \gamma^+(X)$ are equal. It is clear that if two configurations $x$ and $y$ are identical at some common strain $\gamma$, since the AQS dynamics is deterministic, for each value of the strain in the stability interval the particle configurations will be identical and thus $\gamma^\pm(X) = \gamma^\pm(Y)$.

In our numerical implementation, we verify the equality of two mesostates by checking the equality of their stability interval and also comparing the changes in the stress and energy that occur during the plastic transitions at the two ends of the stability interval. This is numerically less costly than evolving two associated particle configurations to some common strain and then checking for their equality. In fact, we found that for the precision of strain $\Delta\gamma$ used, checking just for the equality of the stability intervals suffices.

### S1.3 Construction of the mesostate transition graph

We start with a particle configuration $o$ mechanically stable at zero strain that is obtained by quenching from the high temperature liquid state. We denote the mesostate containing $o$ the reference configuration (RC) and label it as $O$. We then numerically perform the $U$ and $D$ mesostate transitions occurring at $\gamma^+(O)$ and $\gamma^-(O)$, respectively, identifying the resulting mesostates. We continuing then by executing the mesostate transitions from the newly obtained mesostates, each time taking care to identify mesostates that were previously obtained. In this way we ultimately obtain a catalog of mesostates that transit among each other. From this catalog one can construct the mesostate transition graph, as explained in the paper and illustrated by an example in Section S1.4. We describe next the algorithm we used to assemble the catalog of mesostates. In practice, we limit the size of the catalog by restricting it to the set of mesostates that can be reached from the RC by at most $\ell$ transitions. For the data set used in the paper $\ell = 25$.

We give each mesostates an integer ID $0, 1, 2, \ldots,$, and call this the mesostate index. The reference state $O$ has index 0. Our algorithm for assembling the mesostate catalog uses the following variables:

- $n(X)$ - index of mesostate $X$.
- $n_D(X)$ - index pointing to the mesostate obtained from $X$ by shearing in the negative direction, a $D$-transition.
- $n_U(X)$ - index pointing to the mesostate obtained from $X$ by shearing in the positive direction, a $U$-transition.
- $g(X)$ - generation number of mesostate $X$.
- $\gamma^+(X)$ - maximal strain at which mesostate $X$ is stable.
- $\gamma^-(X)$ - minimal strain at which mesostate $X$ is stable.
- $\mathcal{C}$ - catalog of mesostates obtained so far.
- $\ell$ - maximum number of transitions.

When $n_D(X)$ or $n_U(X)$ are NULL, this means that the entries have not been determined yet.

The following is a pseudo-code representation of the algorithm for assembling the mesostate catalog:

set $A = O$
**while** $g(A) < \ell$ **do**
**if** $n_D(A) =$ NULL **then**
find $(\gamma^-(B), \gamma^+(B))$, where $B$ is the mesostate obtained from $X$ by shearing in the negative direction.
set $g(B) = g(A) + 1$
set $n_D(B) =$ NULL
set $n_U(B) =$ NULL
**if** $(\gamma^-(B), \gamma^+(B)) = (\gamma^-(Z), \gamma^+(Z))$ for some existing mesostate $Z \in \mathcal{C}$ **then**
set $n_D(A) = n(Z)$
**else**
add $B$ to $\mathcal{C}$
**end if**
**end if**
**if** $n_U(A) =$ NULL **then**
find $(\gamma^-(C), \gamma^+(C))$, where $C$ is the mesostate obtained from $X$ by shearing in the positive direction.
set $g(C) = g(A) + 1$
set $n_D(C) =$ NULL
set $n_U(C) =$ NULL
**end if**
**if** $(\gamma^-(C), \gamma^+(C)) = (\gamma^-(Z), \gamma^+(Z))$ for some existing mesostate $Z \in \mathcal{C}$ **then**
set $n_U(A) = n(Z)$
**else**
add $C$ to $\mathcal{C}$
**end if**
find mesostate A in $\mathcal{C}$ that has $n_D(A) =$ NULL or $n_A(U) =$ NULL
**end while**

### S1.4: Step by step example of catalog assembly algorithm and mesostate transition graph construction

To illustrate the procedure of catalog assembly and transition graph construction, we show below the different steps of catalog assembly for $\ell = 3$. For each step we present the network and the corresponding state of the catalog table.

- **Initial step:** Initially our catalog only contains the reference configuration $O$ which we index as $n = 0$ and for which we already identified its stability interval $\gamma^{\pm}(O)S$. The mesostates obtained from a $D$ or $U$ transitions out of $O$ have not been extracted yet, so their indices $n_U$ and $n_D$ are still undetermined and hence NULL. The generation number of $O$ is $g = 0$:

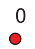


| $n$ | $n_D$ | $n_U$ | $g$ | $\gamma^-$ | $\gamma^+$ |
|---|---|---|---|---|---|
| 0 | NULL | NULL | 0 | -0.0107 | 0.0231 |

- **Step 1:** Our catalog contains meso-states whose generation $g$ is less equal $\ell = 3$ and for which the $D$ transitions have not been determined yet. We numerically determine the mesostate resulting from the $D$-transition of mesostate $n = 0$. We identify this as a new meso-state, give it the index $n = 1$, assign it to generation $g = 1$, and extract its stability interval. We add a new entry for this mesostate into our catalog and update the $n_D$ entry for 0:

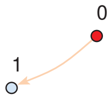


| $n$ | $n_D$ | $n_U$ | $g$ | $\gamma^-$ | $\gamma^+$ |
|---|---|---|---|---|---|
| 0 | 1 | NULL | 0 | -0.0107 | 0.0231 |
| 1 | NULL | NULL | 1 | -0.0297 | 0.0204 |

- **Step 2:** We work out the $U$ mesostate transition from 0, leading to a new mesostate with index $n = 2$:

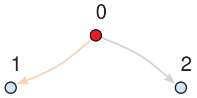


| $n$ | $n_D$ | $n_U$ | $g$ | $\gamma^-$ | $\gamma^+$ |
|---|---|---|---|---|---|
| 0 | 1 | 2 | 0 | -0.0107 | 0.0231 |
| 1 | NULL | NULL | 1 | -0.0297 | 0.0204 |
| 2 | NULL | NULL | 1 | -0.007 | 0.0367 |

- **Step 3:** The $D$-transition from mesostate $n = 1$ leads to a new mesostate, belonging to generation $g = 2$, that we index as 3:

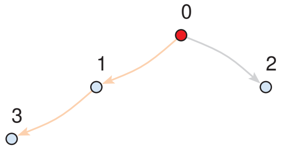


| $n$ | $n_D$ | $n_U$ | $g$ | $\gamma^-$ | $\gamma^+$ |
|---|---|---|---|---|---|
| 0 | 1 | 2 | 0 | -0.0107 | 0.0231 |
| 1 | 3 | NULL | 1 | -0.0297 | 0.0204 |
| 2 | NULL | NULL | 1 | -0.007 | 0.0367 |
| 3 | NULL | NULL | 2 | -0.0366 | 0.004 |

- **Step 4:** The $U$-transition from mesostate $n = 2$ leads to to a new mesostate that we index as 4:

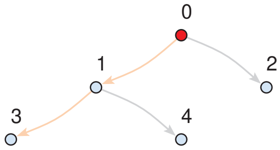


| $n$ | $n_D$ | $n_U$ | $g$ | $\gamma^-$ | $\gamma^+$ |
|---|---|---|---|---|---|
| 0 | 1 | 2 | 0 | -0.0107 | 0.0231 |
| 1 | 3 | 4 | 1 | -0.0297 | 0.0204 |
| 2 | NULL | NULL | 1 | -0.007 | 0.0367 |
| 3 | NULL | NULL | 2 | -0.0366 | 0.004 |
| 4 | NULL | NULL | 2 | -0.0318 | 0.0355 |

- **Step 5:** The $D$-transition from mesostate $n = 2$ leads to a mesostate that we have already identified as part of our catalog with index 4:

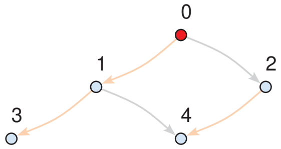


| $n$ | $n_D$ | $n_U$ | $g$ | $\gamma^-$ | $\gamma^+$ |
|---|---|---|---|---|---|
| 0 | 1 | 2 | 0 | -0.0107 | 0.0231 |
| 1 | 3 | 4 | 1 | -0.0297 | 0.0204 |
| 2 | 4 | NULL | 1 | -0.007 | 0.0367 |
| 3 | NULL | NULL | 2 | -0.0366 | 0.004 |
| 4 | NULL | NULL | 2 | -0.0318 | 0.0355 |

- **Step 6:** The $U$-transition from mesostate $n = 2$ leads to a new mesostate that we index as 5:

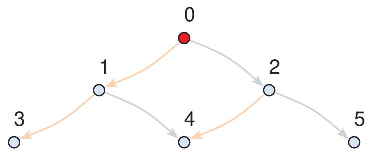


| $n$ | $n_D$ | $n_U$ | $g$ | $\gamma^-$ | $\gamma^+$ |
|---|---|---|---|---|---|
| 0 | 1 | 2 | 0 | -0.0107 | 0.0231 |
| 1 | 3 | 4 | 1 | -0.0297 | 0.0204 |
| 2 | 4 | 5 | 1 | -0.007 | 0.0367 |
| 3 | NULL | NULL | 2 | -0.0366 | 0.004 |
| 4 | NULL | NULL | 2 | -0.0318 | 0.0355 |
| 5 | NULL | NULL | 2 | 0.0162 | 0.0432 |

Note that if we had set $\ell = 2$, our catalog would be completed, since we have identified all the mesostate transitions involving the states with $g < 2$. We show next a few more steps and then the final step when the catalog at $\ell = 3$ is complete:

- **Step 7:**

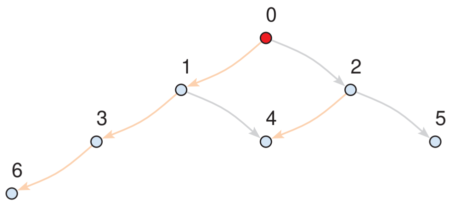


| $n$ | $n_D$ | $n_U$ | $g$ | $\gamma^-$ | $\gamma^+$ |
|---|---|---|---|---|---|
| 0 | 1 | 2 | 0 | -0.0107 | 0.0231 |
| 1 | 3 | 4 | 1 | -0.0297 | 0.0204 |
| 2 | 4 | 5 | 1 | -0.007 | 0.0367 |
| 3 | 6 | NULL | 2 | -0.0366 | 0.004 |
| 4 | NULL | NULL | 2 | -0.0318 | 0.0355 |
| 5 | NULL | NULL | 2 | 0.0162 | 0.0432 |
| 6 | NULL | NULL | 3 | -0.0456 | 0.0057 |

- **Step 8:**

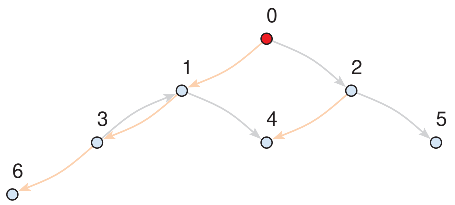


| $n$ | $n_D$ | $n_U$ | $g$ | $\gamma^-$ | $\gamma^+$ |
|---|---|---|---|---|---|
| 0 | 1 | 2 | 0 | -0.0107 | 0.0231 |
| 1 | 3 | 4 | 1 | -0.0297 | 0.0204 |
| 2 | 4 | 5 | 1 | -0.007 | 0.0367 |
| 3 | 6 | 1 | 2 | -0.0366 | 0.004 |
| 4 | NULL | NULL | 2 | -0.0318 | 0.0355 |
| 5 | NULL | NULL | 2 | 0.0162 | 0.0432 |
| 6 | NULL | NULL | 3 | -0.0456 | 0.0057 |

- **Final step:** Below is the complete catalog and transition graph at $\ell = 3$:

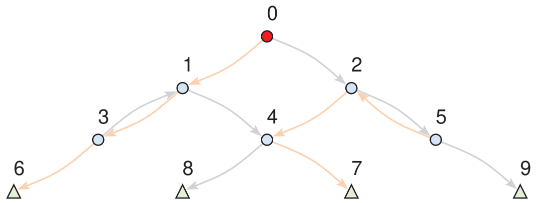


| $n$ | $n_D$ | $n_U$ | $g$ | $\gamma^-$ | $\gamma^+$ |
|---|---|---|---|---|---|
| 0 | 1 | 2 | 0 | -0.0107 | 0.0231 |
| 1 | 3 | 4 | 1 | -0.0297 | 0.0204 |
| 2 | 4 | 5 | 1 | -0.007 | 0.0367 |
| 3 | 6 | 1 | 2 | -0.0366 | 0.004 |
| 4 | 7 | 8 | 2 | -0.0318 | 0.0355 |
| 5 | 2 | 9 | 2 | 0.0162 | 0.0432 |
| 6 | NULL | NULL | 3 | -0.0456 | 0.0057 |
| 7 | NULL | NULL | 3 | -0.0473 | 0.0019 |
| 8 | NULL | NULL | 3 | 0.0149 | 0.0416 |
| 9 | NULL | NULL | 3 | 0.0019 | 0.0496 |

Note that the catalog is complete at $\ell = 3$, since for all states with $g < \ell$ we have identified the mesostates they transit to and thus the catalog entries for these states have all non-NULL entries in their $n_D$ and $n_U$ columns. We call

the states with $g = \ell$ the peripheral states. For these the entries for $n_D$ and $n_U$ will be `NULL`. In the transition graph we mark the vertices corresponding to peripheral states by green triangles.

## S2 SUPPORTING EVIDENCE

We present here supporting evidence for the claim that the features observed in the paper persist qualitatively when considering a larger number of particles, Section S2.1, or investigating limit cycles at moderately high strain amplitude relative to yield, Section S2.2.

### S2.1 Mesostate transition graph for a system of $N = 4096$ particles

The numerical results discussed in the paper involve a system of $N = 1024$ particles, leading at $\ell = 25$ to a catalog of $\mathcal{N} = 1416$ mesostates. In the paper we observed that the mesostate transition graph has tree-like features as well as regions with high interconnections. The top panel (a) of Fig. 1 below depicts this transition graph. It is a blown-up and rescaled version of Figure 1(b) of the paper. The graph contains regions with high interconnectivity as well as tree-like regions that we have highlighted in blue. In particular there are bottleneck regions where one-way transitions connect one part of the graph with another. Some one-way transitions making up the bottleneck have been highlighted in green. At the catalog size we considered there does not appear to be any transition back to the other side of the bottleneck. The reference configuration of this catalog has been marked in red and labeled by $O$. The dashed arrows connecting the vertices in dark blue indicate the transient leading to a limit cycle (solid black and red transitions) that is obtained when starting at $O$ and oscillatory shear at strain amplitude $\gamma = 0.0500$ is applied.

The bottom panel (b)of Fig. 1 shows the mesostate transition network obtained numerically from a reference configuration $O$ for a system of $N = 4096$ particles, using again $\ell = 25$. The catalog contains $\mathcal{N} = 1525$ mesostates. The transition graph is qualitatively similar to that obtained for the $N = 1024$ particle system shown in (a). It contains bottleneck regions (shown in green) as well as tree-like features some of which are highlighted in blue. The transient and limit-cycle shown in the figure were obtained applying oscillatory shear at amplitude $\gamma = 0.0320$ to $O$. We have also checked and found that in this limit cycle which includes 34 mesostates, there are only two RPM violations no rabbit-holes which is similar to what we observed for the system with $N = 1024$ particles.

### S2.2 Mesostate transition graph associated with limit-cycles at larger strain amplitudes

Here we provide additional evidence that limit-cycles reached at moderately large strain amplitudes relative to yield, still exhibit relatively few RPM violating transitions and rabbit holes. Figure 2 of the paper shows the state transition graph containing the limit-cycle that is reached when starting at $O$ and applying oscillatory shear at strain amplitude $\gamma = 0.0500$. The yielding strain for our sample was determined to be $\gamma_y = 0.13$. Here we consider the limit cycle that is reached when starting from the same reference configuration $O$ oscillatory shear at an amplitude $\gamma = 0.0830$ is applied. This limit cycle is established by the end of the second driving period. Since at larger amplitudes there are more plastic events making up the limit cycle, we assembled a catalog of mesostates at $\ell = 36$. Despite of the larger $\ell$ used, we captured only part of the limit cycle, as depicted in Fig. 2. The mesostate labeled $\mathbf{O}'$ is the zero strain state of the $\gamma = 0.0830$ limit-cycle. More precisely, $O'$ is the mesostate on the limit cycle reached when the strain is rising from $-0.0830$ to zero. The cycle with endpoints $(\mathbf{X}, \mathbf{Y})$ shown in the figure is a sub-cycle of this limit cycle that will be traced out when starting in $\mathbf{O}'$ the strain is first raised to a value 0.0722 (state $\mathbf{Y}$), then lowered to $-0.0830$ (state $\mathbf{X}$), then back up to 0.0722 *etc.* Two sub-cycles of this cycle are shown in the figure (shaded in green) along with the range of strains at which the associate mesostates are confined to these cycles.

The state transition graph shown in the figure contains 207 mesostates and 412 transitions. Out of these only 17 transitions turn out to be RPM violating. These have been highlighted by thicker black and red arrows. Note that most of these RPM violations occur in the highlighted sub-cycle containing the upper endpoint $\mathbf{Y}$. Note also that this limit cycle does not contain rabbit-hole transitions.

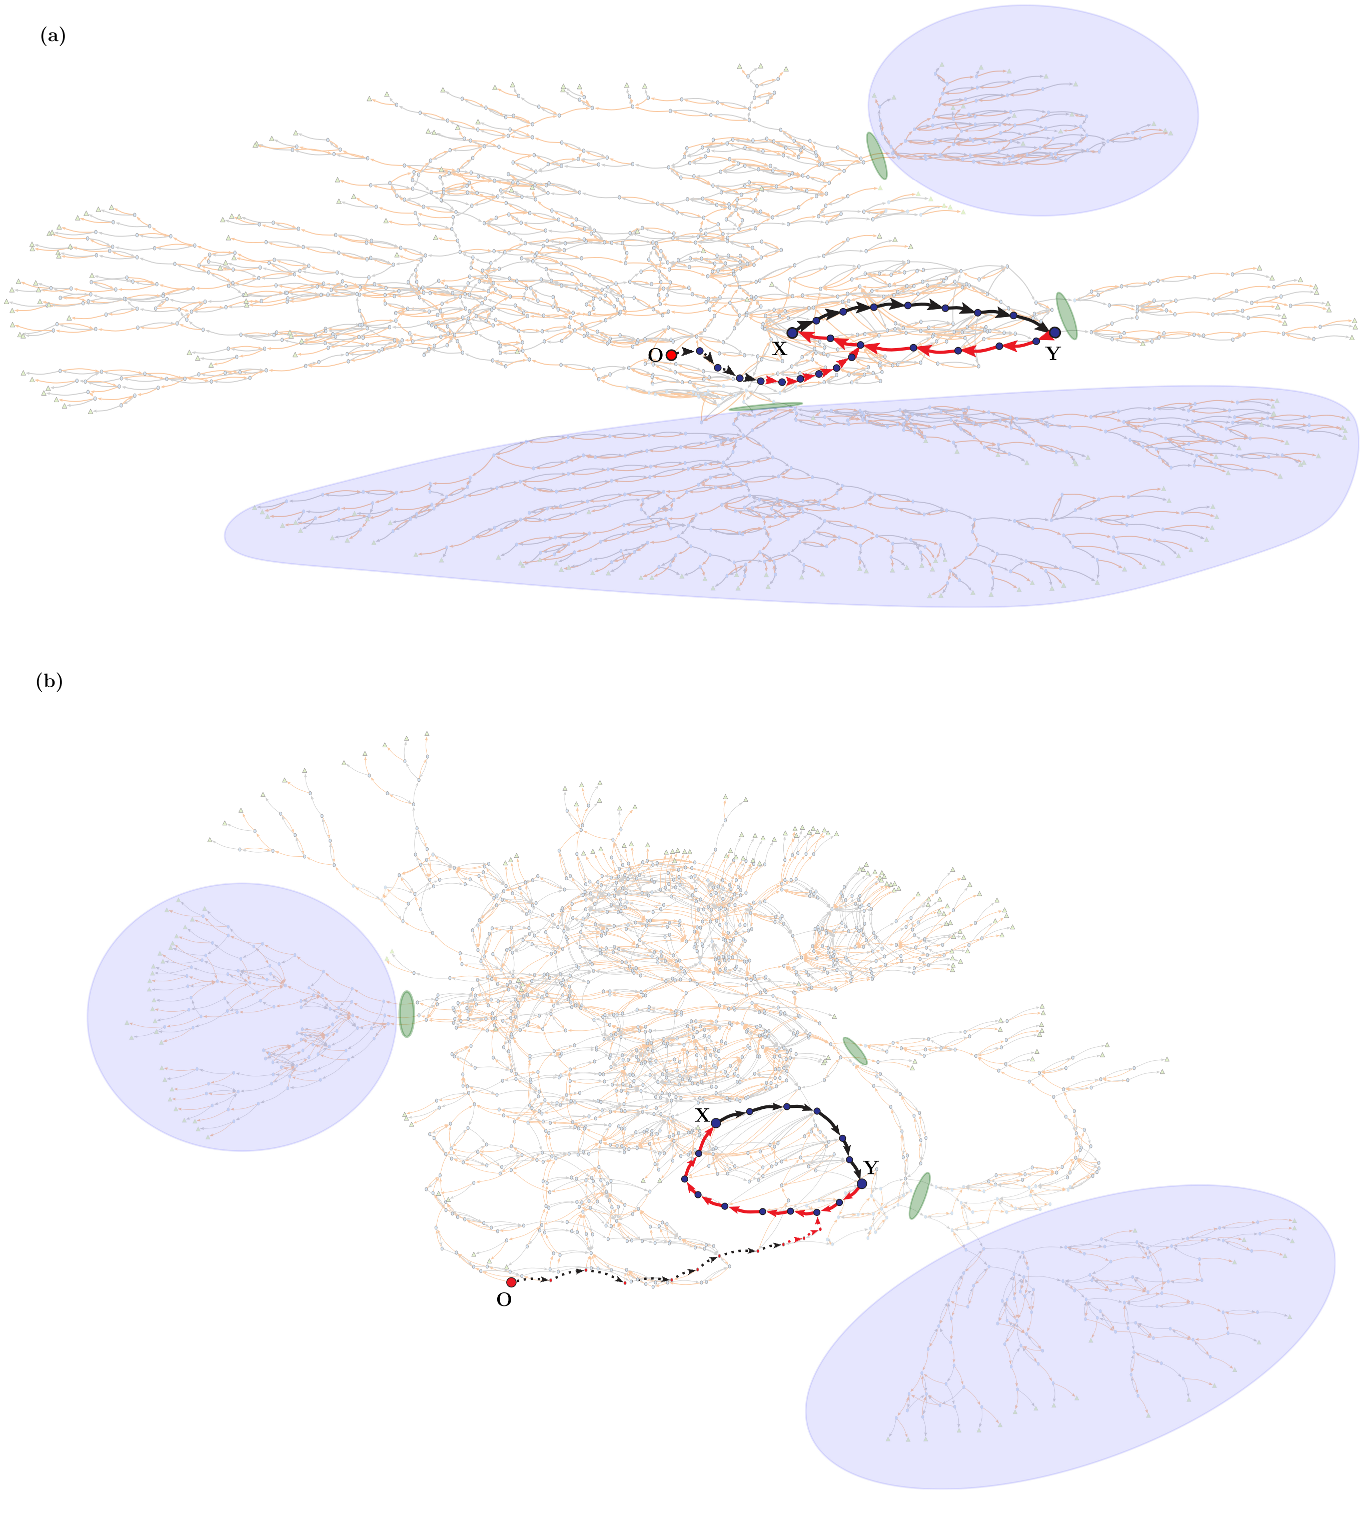


FIG. 1. (color online) Comparing the mesostate transition graph obtained from numerical simulations of a sheared amorphous solid with $N = 1024$ (a) and $N = 4096$ (b) particles. Both graphs exhibit qualitatively similar features of tree-like regions (shaded in blue) and bottle-necks (shaded in green). Refer to text for further details.

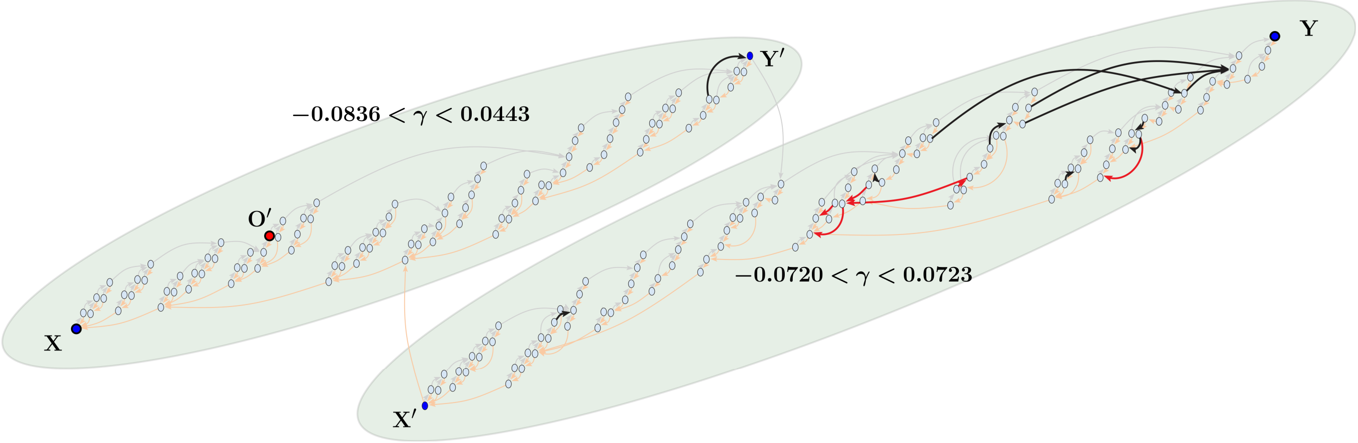


FIG. 2. (color online) Mesostate transition graph associated with the limit-cycle reached when oscillatory shear at amplitude $\gamma = 0.0830$ is applied. The transition graph shown contains 207 mesostates and 412 transitions and is a sub-cycle of the full limit-cycle Refer to text for further details.
